# Supplementary material for: On the miscibility gap of Cu-Ni system
Source: arXiv:1611.07068 source file (2016-11-28)
Supplement: Supplementary file 1 [file _auto-ignoreSupplementaryMaterial.pdf]

# Supplementary Material: On the miscibility gap of Cu-Ni system

Yusuke Iguchi,[1,a] Gábor Katona,[1] Csaba Cserháti,[1] Gábor Langer,[1] and Zoltán Erdélyi[1,b]

*Department of Solid State Physics, University of Debrecen, Bem ter 18/b., Debrecen, H-4026 HUNGARY*

(Dated: 21 November 2016)

PACS numbers: 81.30.Bx, 64.75.St, 82.80.Ms, 66.30.Pa

Keywords: phase diagram, thin films, secondary neutral mass spectroscopy (SNMS), diffusion

[a] Corresponding author: iguchi.yusuke@atomki.mta.hu; Present Affiliation: Institute for Nuclear Research, Hungarian Academy of Sciences, Bem ter 18/c., Debrecen, H-4026 HUNGARY

[b] http://web.unideb.hu/zerdelyi

## SAMPLE PREPARATION

Various Cu/Ni thin films were deposited onto oxidized silicon substrates by DC magnetron sputtering at room temperature. The base pressure of the sputtering chamber was lower than $5 \times 10^{-4}$ Pa. During the deposition of copper and nickel layers the Ar (99.999 %) pressure (under dynamic flow) and the sputtering power were $5 \times 10^{-1}$ Pa and 40 W, respectively. Purities of Cu and Ni targets were 99.99 and 99.995%, respectively. The deposition rates were calibrated using Ambios XP-1 profilometer as 0.5 nm/s for Cu and 0.25 nm/s for Ni.

## SECONDARY NEUTRAL MASS SPECTROMETRY AND PROFILE RECONSTRUCTION

The time evolution of the diffusion process occurring after heat treatments in Cu-Ni film was determined by an INA-X type SNMS ( SPECS GmbH, Berlin) equipment. In this instrument, low pressure HF plasma ($10^{-1}$ Pa) is used as ion source as well as post ionization medium for the sputtered neutrals. Due to the low pressure in the plasma chamber the interactions (chemical, scattering) between sputtered particles and working gas are negligible. As the emission and the ionization process of the analyzed particles are decoupled in SNMS, the post-ionization probability is practically determined by the experimental arrangement (plasma parameters) and therefore largely independent on the target composition[1]. Consequently, the SNMS signal $I(X)$ of species $X$ depends on only its composition in the target and the total sputter yield. This is the basis of the quantification of SNMS measurement. Details of quantification is described in[2]. In the INA-X type SNMS extremely plane bombarding craters are obtained when the bombarding voltage (typically few hundred eV), the plasma parameters and plasma - sample distance are chosen appropriately. As a result, high depth resolution of the order of $1 - 2$ nm can be achieved and maintained over few hundred nm sputtered depth.

The SNMS measurements give us the information with intensity-time profiles. These were converted to composition – depth profiles using relative sensitivity factors assuming linear dependence of the intensity and local density on concentration[3]. The total sputtered depth was determined by Ambios XP-1 profilometer.

The detection limit of an element in a matrix is less than 100 ppm with around 2nm

depth resolution. However after the conversion from the time to depth, the determination of the atomic fraction from the measured intensities has an uncertainty of around $\pm 2at\%$, empirically. Smoothing using Savitzky-Golay filter was applied to all of the converted depth profiles.

## HEAT TREATMENTS WITH ERRORS OF TEMPERATURE MEASUREMENTS

The temperature of the heating unit, which was a stainless steel stage heated with a halogen lamp, was controlled by commercial sheathed K-type thermocouple. It was located at the edge of the heating stage with the distance of 2 to 3 cm from the sample.

The sample on the heating stage was pinched by mica and stainless steel plate, and it was also covered by thermal reflectors to prevent the heat radiation loss. In case of K-type thermocouple there is a well-known issue: short range ordering in the thermocouple can cause drift of +1 to 5 K in a few minutes to a month in the range from 523 to 823 K (e.g.[4,5]). This range and drift value are unclear and somewhat different in different literature. To guarantee that the annealing temperature on the top of the thin film is the desired one, we calibrated the K-type thermocouple with the help of a non-sheathed J-type thermocouple which was located on the surface of a phantom sample.

Figure 1 shows the temperature difference between the heating stage and sample top. Empirically, the error between the heating unit and actual temperature of the samples was about ±2% in the temperature range of 673 to 823 K; which was the temperature range in this study. The heat treatments at a given temperature were done sequentially using the same piece of sample until reaching equilibrium (no change on the composition profile even after multiplying the annealing time). The time to reach the thermodynamic equilibrium (steady state) was—depending on the temperature and thickness— about 1 week in this study.

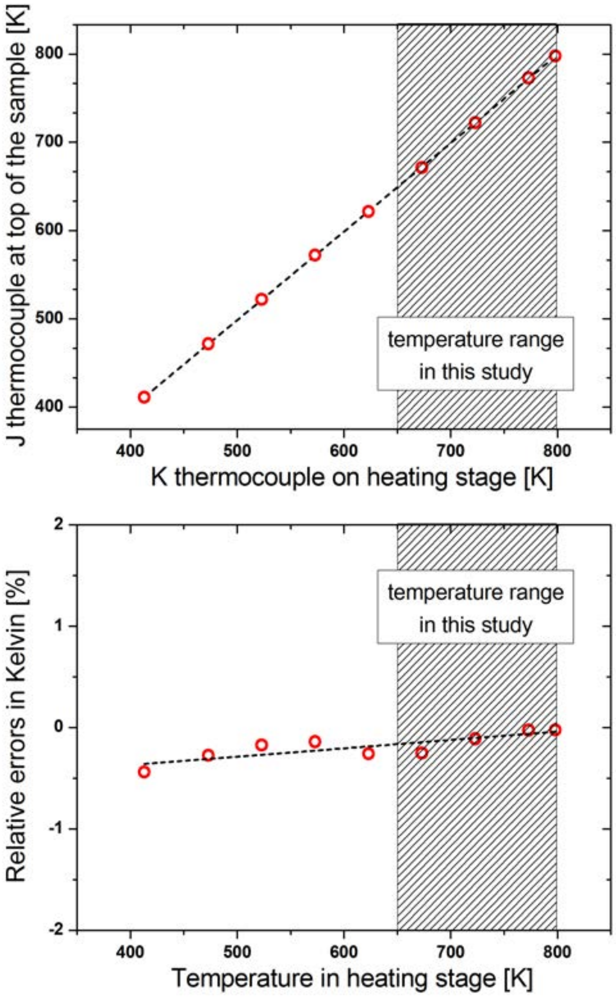


FIG. 1. Upper panel: temperature difference between the heating stage and the top of the sample. Lower panel: relative error between the sample and the stage.

## MORPHOLOGY OF THE REACTION ZONE IN THE NANO-DIFFUSION COUPLE TECHNIQUE

We performed X-TEM experiments, in order to collect more information about the samples morphology. On Figure 2.a. an X-TEM BFI image of the as deposited sample is presented. The picture shows the usual columnar Cu-grains perpendicular to the surface and small Ni-grains at the substrate side (sample type (c)). On Fig 2.b. and c. a BFI and a DFI image of an annealed sample is displayed. These images are corresponding to the SNMS profiles drawn on Figure 2 in the main manuscript.

On Figure (Fig.2.b) one can see grains with a size comparable of the total film thickness.

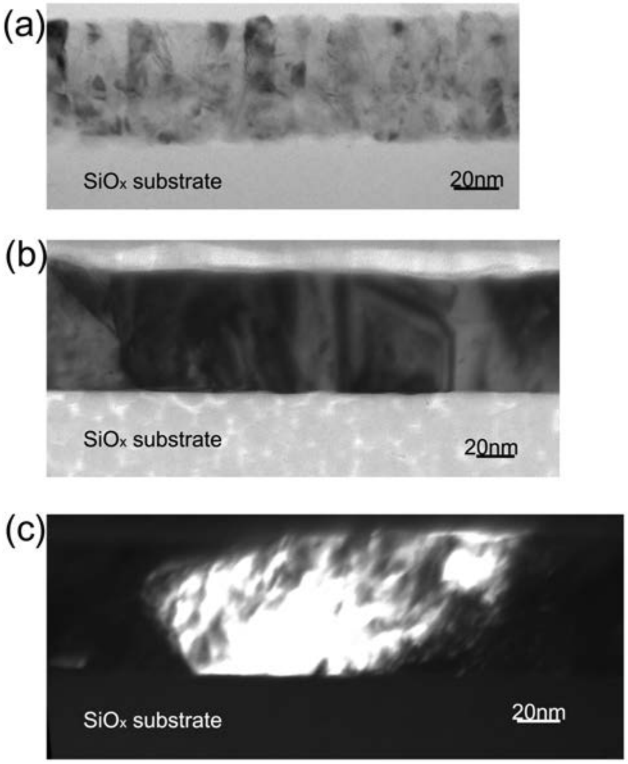


FIG. 2. Cross-section TEM pictures of sample type (c) $Cu_{31nm}/Ni_{29nm}/SiO_x$ (Ni average composition 50 at%; total film thickness 60 nm), (a) Bright Field Image of as-deposited, (b) Bright Field Image of annealed at 725K for 7 days, and (c) Dark Field Image of annealed at 725K for 7 days.

Relatively huge and continuous grains growing along to the surface from the substrate was observed in the BFI and DFI of TEM after annealing, Fig.2. (b) and (c). There are neither distinct phases, nor indications of DIR/DIGM. It has to be mentioned, that there is no atomic contrast due to the similar atomic properties of the constituents. These images also suggest, that diffusion induced stress effects are negligible.

Interdiffusion in this study show type-A grain boundary diffusion because the lattice diffusion length in these experiments is larger than the grain boundary with[6,7] which is to use diffusion parameter from[8]. Diffusion length $2\sqrt{Dt}$ of Ni into Cu, as an example, is about 50nm at 722K for 48h[9], which is larger than the grain boundary width (0.5nm[8]).

Effective diffusion coefficient of type-A diffusion, which has an almost planar diffusion front, represents a weighted average of the volume and grain-boundary diffusivity i.e. it is much faster than bulk diffusion only. This fast diffusivity on this length-scale is advantageous to apply for the determination of the equilibrium state. Since the diffusion length is the same

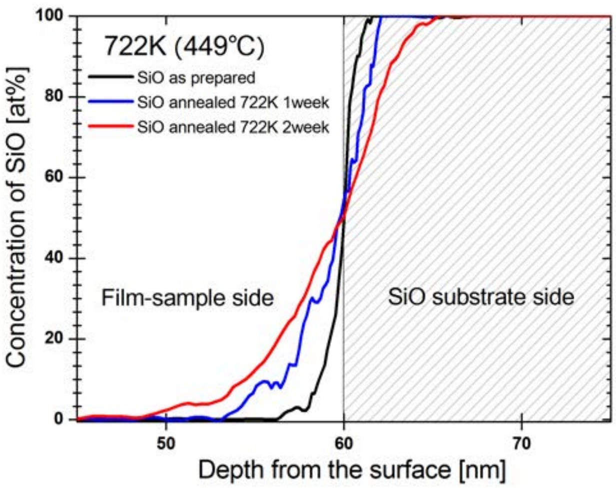


FIG. 3. SNMS around interface between of sample type (c) $Cu_{31nm}/Ni_{29nm}/SiO_x$ (Ni average composition 50 at%; total film thickness 60 nm), (a) as prepared, (b) annealed at 722K for 7 days, and (c) annealed at 722K for 14 days.

for the thinner bi as well as the thicker trilayered samples on the same temperature, the time to reach the equilibrium is much longer for the thicker sample. Note, that during the annealing, grain coarsening happened (see the TEM images above), which means that the weight of the grain boundary diffusion decreases with the annealing time, i.e the diffusion slows down, which also increases the time to reach the equilibrium for the thicker samples.

## DETERIORATION OF THE DEPTH RESOLUTION DUE TO LONG-TERM HEAT TREATMENT: TECHNICAL ISSUES OF SPUTTERING MEASUREMENT

Additionally, long time annealing can cause bad depth resolution of the SNMS measurement due to surface roughing caused by grain coarsening[10,11]. Figure 3 shows how the shape of the interface, at CuNi/SiO substrate, changes with annealing time. Note, that the interface after 1 week annealing is about 2, after 2 weeks annealing is about 3 times wider than the as-prepared one. In our opinion it is not due to Si diffusion into the film, but because the rough/wavy top surface comes down during plasma sputtering. TEM pictures in Fig.2. also supports that the interface is indeed sharp, so the widening is an artifact which comes from the method. This also shows the limits of the method, i.e. interface profiling of thin films

by SNMS or by other sputtering method does not give satisfactory results after too long annealing. Based on this experience, we decided only for 1 week annealing as an optimum.

This work was supported in part by the OTKA Board of Hungary (No. NF101329) and by TAMOP 4.2.2.A-11/1/KONV- 2012-0036 project (implemented through the New Hungary Development Plan co-financed by the European Social Fund, and the European Regional Development Fund). Y. I. acknowledge the support from Hungarian Academy of Sciences Postdoctoral Fellowship Programme.

## REFERENCES

[1]H. Oechsner and E. Stumpe, Appl. Phys. **14**, 43 (1977).

[2]H. Oechsner., Nucl. Instrum. Methods. Phys. Res. B **33**, 918 (1988).

[3]A. Wucher and H. Oechsner., Z. Anal. Chem. **333**, 470 (1989).

[4]A. Fenton, *Proc. 5th Symp. on Temperature Washington DC (June 21-2-24 1971) Inst. Soc. of Am*, , 1973 (1971).

[5]R. E. Bentley, Sensors and Actuators A Physical , 2421 (1990).

[6]I. V. Belova and G. E. Murch, Philos. Mag. A **81**, 2447 (2001).

[7]H. Mehrer, *Diffusion in Solids: Fundamentals.* (Springer, 2007).

[8]H. Mehrer, *Diffusion in Solid Metals and Alloys, Landolt-Börnstein, New Series, Group III: Crystal and Solid State Physics, Vol. 26.* (Springer, 1990).

[9]G. Neumann and V. Tölle., Philos. Mag. A **57**, 621 (1988).

[10]T. Wöhner and et al., Surf. Interface Anal. **26**, 1 (1998).

[11]P. Sophia and et al., ESC J. Solid State Sci. Technol **4**, 53 (2015).
